# Supplementary material for: Towards glasses with permanent stability
Source: arXiv:2011.09259 ancillary file (2021-11-24)
Supplement: Supplementary file 1 [file Supplemental.pdf]

# Supplemental Material for “Towards Glasses with Permanent Stability”

Taiki Yanagishima,<sup>1,2</sup> John Russo,<sup>3</sup> Roel P. A. Dullens,<sup>1</sup> and Hajime Tanaka<sup>4,5,\*</sup>

<sup>1</sup>*Department of Chemistry, Physical and Theoretical Chemistry Laboratory,  
University of Oxford, South Parks Road, OX1 3QZ, United Kingdom*

<sup>2</sup>*Department of Physics, Graduate School of Science, Kyoto University, Kyoto, 606-8224, Japan*

<sup>3</sup>*Department of Physics, Sapienza University of Rome, P. le Aldo Moro 5, 00185 Rome, Italy*

<sup>4</sup>*Department of Fundamental Engineering, Institute of Industrial Science,  
University of Tokyo, 4-6-1 Komaba, Meguro-ku, Tokyo 153-8505, Japan*

<sup>5</sup>*Research Center for Advanced Science and Technology,  
University of Tokyo, 4-6-1 Komaba, Meguro-ku, Tokyo 153-8505, Japan*

## DESIGN OF THE UG ALGORITHM

It is a key feature of the UG algorithm that its specific features and details do not significantly affect the reliable production of UG states. Design choices were primarily geared to the rapid, reproducible generation of initial states over a wide range of volume fractions for subsequent scrutiny and numerical propagation. These choices are described here.

Reviewing the method, we start from a configuration randomly generated using a modified Lubachevsky-Stillinger algorithm [1]. This is FIRE [2] minimized to produce a conventional glass (CG) state. We apply a radical Voronoi tessellation to identify inhomogeneities and find where particle sizes need to be adjusted. Particle diameters are adjusted, then particles are replaced in the center of each Voronoi cell. The intention of both actions is to reduce volume fraction inhomogeneities, though the latter is only significant at low volume fractions when Voronoi cells can be more empty; either way, note that the newly generated configuration has a different Voronoi diagram AND is no longer at a local energy minimum (albeit not by much). Different design choices, for example, using a non-radical, normal Voronoi diagram, not replacing particles in Voronoi cell centers, or adjusting particle sizes in smaller steps (e.g., a fraction of the intended size correction), have little effect except to slow down the convergence rate of  $\Delta\phi_i/\langle\phi_i\rangle$ . The bottom line is that all steps modify the energy landscape, which requires a configurational update. The algorithm intrinsically drives the state out of equilibrium.

Also, note that we have chosen to select a monotonic decay in  $\Delta\phi_i/\langle\phi\rangle$ , reducing the magnitude of size corrections until some convergence is reached. This need not be the case; continuing to apply the same algorithm does indeed result in configurations with even lower  $\Delta\phi_i/\langle\phi_i\rangle$ . However, as shown in Fig. S1, the trajectory becomes oscillatory, largely due to the feedback loop between size updates and successive energy minimizations described above. Taking all this into account, however, it should be stressed that the key transition to aging-free behavior described in the paper is seen *significantly* before this, after only a few iterations of the algorithm.

As a point of discussion, if we were to try to achieve strongly hyperuniform configurations via some variant on this method, we should note that all moves made here are all collective, i.e., applied to all particles at once. Local moves that, e.g., make adjustments to a single randomly chosen particle may be more suitable, much like in Monte Carlo simulations where moves become rarer with density. To achieve a significant reduction in  $\Delta\phi_i/\langle\phi_i\rangle$ , however, would require orders of magnitude more applications of the FIRE algorithm, which leads to prohibitively long computation times. A more efficient formulation, e.g., selecting for notably large inhomogeneities and a faster computational engine such as a GPU implementation of FIRE may ultimately lead to hyperuniform packings of this variety.

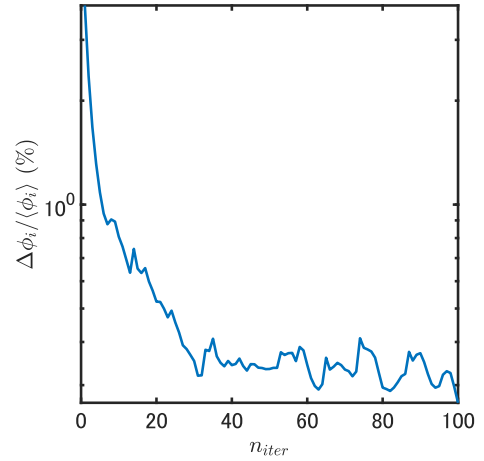

FIG. S1. Evolution of  $\Delta\phi_i/\langle\phi_i\rangle$  with iterations of the algorithm that generates UG states.

## RADIAL DISTRIBUTION FUNCTION

We examine the structural changes that occur going from CG to UG states by the radial distribution function  $g(r)$ . Figure S2 plots  $g(r)$  for CG, UG, and re-CG states, showing that the  $g(r)$  of UG and re-CG states

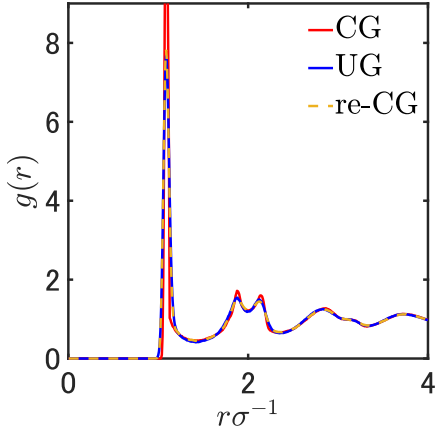

FIG. S2. Radial distribution  $g(r)$  of CG, UG and re-CG states, averaged over 50 independently generated configurations. UG and re-CG states have virtually identical  $g(r)$ , showing that the only impact on  $g(r)$  comes purely from polydispersity.

(which have the same particle-size distribution) are almost indistinguishable. Pair correlations thus are unable to capture the sharp discrepancy between the dynamics of UG and re-CG states.

### COMPRESSIBILITY OVER ITERATINOS

We also look at the compressibility factor  $Z = \beta P_V / \langle \sigma^3 \rangle$  over the course of the iterations, where  $P_V$  is the virial pressure; 20 independent examples of how  $Z$  evolves with the dispersion in  $\phi_i$ ,  $\Delta\phi_i / \langle \phi_i \rangle$ , are shown in Fig. S3. There is a systematic reduction in  $Z$  with successive steps, despite the minimal changes to nearest neighbor bond-orientational order (see Fig. 4(a)). Taken together, this suggests that this is not a state which is reached thermodynamically.

### UG GLASSES AT DIFFERENT VOLUME FRACTIONS

In Fig. S4, we plot the local volume fraction  $\phi_i^{\text{eff}}$  dependence of the average number of force neighbors  $\langle n_{\text{FN}} \rangle$  for different values of the average volume fraction  $\phi_0$ . The UG algorithm produces sharper  $\phi_i^{\text{eff}}$  distributions for higher  $\phi_0$ ;  $\Delta\phi_i / \langle \phi_i \rangle$  is approximately 1.9% when  $\phi_0 = 0.60$  compared to 0.56% when  $\phi_0 = 0.69$ , averaged

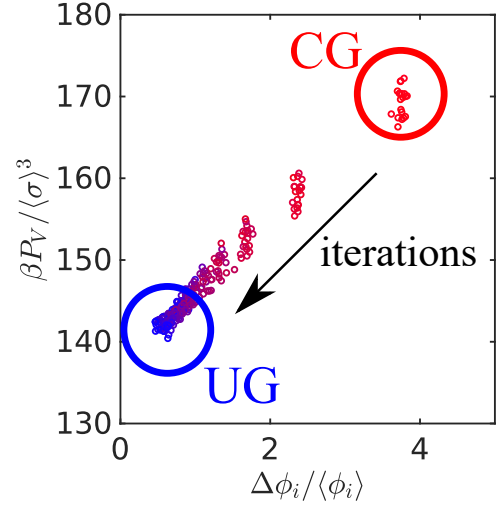

FIG. S3. Change of the compressibility  $Z = \beta P_V / \langle \sigma^3 \rangle$  with iterations over 20 independent runs of the algorithm, going from CG to UG states. There is a progressive reduction.

over 5 states each. Thus, the narrowing in the distribution of  $n_{\text{FN}}$  is less pronounced at lower  $\phi_0$ , suggesting that a more severe homogenization in  $\phi_i^{\text{eff}}$  may be required to achieve similar stabilization at lower  $\phi_0$ .

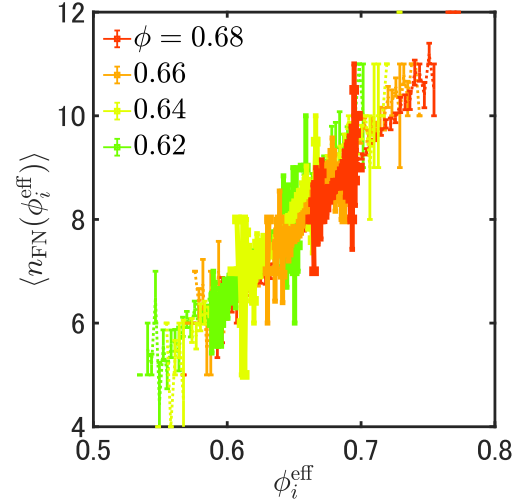

FIG. S4. Number of force neighbors as a function of local  $\phi_i^{\text{eff}}$  for CG and UG states generated at different volume fractions. Number of force neighbors  $\langle n_{\text{FN}} \rangle$  as a function of local effective volume fraction  $\phi_i^{\text{eff}}$  for CG and UG states generated at different global volume fractions. Dotted lines indicate CG states, and thick solid lines indicate the corresponding UG states. All curves show a linear relationship which is preserved going from CG to UG states.

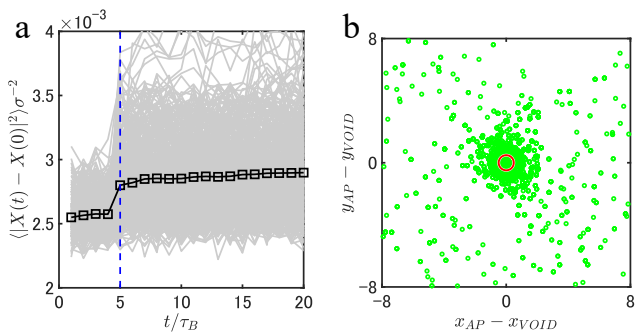

FIG. S5. Artificially triggered avalanches. (a) Squared displacements for when a particle is artificially removed from a UG configuration. Each grey line indicates independent runs when a specific particle is removed at time  $t = 5\tau_B$  (vertical blue dashed line). The black squares and line are the average squared displacement over 400 different choices of particle to remove. (b)  $xy$ -plane projection of avalanche particles (AP; green particles) which have moved over  $\sigma_i/3$  from time  $t = 5\tau_B$  to  $40\tau_B$ . All positions are given relative to the location of the specific particle removed or “voided” at  $t = 5\tau_B$  for each run,  $(x_{VOID}, y_{VOID})$ . Avalanche events are highly localized around the particle removed (marked with a red circle).

#### ARTIFICIALLY TRIGGERED AVALANCHES

Due to the finely balanced nature of the UG state, it would be interesting to observe what would happen if this mechanical balance was locally perturbed. Thus, we take a UG state and artificially remove a single particle. The squared displacement of the configuration for 400 different particle choices is shown in Fig. S5(a), along with the average squared displacement. Note that the particle is removed or “voided” at time  $t = 5\tau_B$ . Indeed, it is clear that an avalanche is artificially triggered at this time, and quickly terminated, though there is a small proportion of runs that go on to trigger other events. An  $xy$ -projection of the location of particles that move significantly (more than  $\sigma_i/3$ ), i.e., take part in avalanches, are shown relative to the particle that is removed in Fig. S5(b). Note how the events are highly

localized to the vicinity of the particle removed; this is in sharp contrast to the widespread collective events seen for avalanches in deeply supercooled glasses [3]. This is largely due to the even distribution of forces throughout the system and thus the extensive connectivity of the force network, which acts to stabilize nearby structures.

#### LEGEND FOR SUPPLEMENTARY MOVIE

Force chain network and crystalline particles (red) in CG and UG states propagated over time using Brownian Dynamics. Frames are rendered every  $10\tau_B$ , with playback set to  $200\tau_B$  per second. Thus, the whole video spans  $4000\tau_B$ . Blue links in the force chain network are preserved compared to an initial state. For the CG state, this is taken early in the first plateau in the squared displacement of the particles. The same initial time is used for the UG state. Red links are broken connections; green links are new connections. While the CG state features permanent re-configurations, with intermittent bursts of rearrangements accompanying crystal growth, the UG states only show small fluctuations. We can see that in the UG state, the ‘skeletal’ parts made of force-bearing bonds making up the majority of the force network are stable, whereas a very small number of weak bonds in the non-skeletal parts occasionally recombine.

---

\* tanaka@iis.u-tokyo.ac.jp

- [1] B D Lubachevsky and F H Stillinger, “Geometric properties of random disk packings,” *J. Stat. Ph* **60**, 561–583 (1990).
- [2] E. Bitzek, P. Koskinen, F. Gähler, M. Moseler, and P. Gumbsch, “Structural relaxation made simple,” *Phys. Rev. Lett.* **97**, 170201 (2006).
- [3] E Sanz, C Valeriani, E Zaccarelli, W C K Poon, Michael E Cates, and P N Pusey, “Avalanches mediate crystallization in a hard-sphere glass,” *Proc. Natl. Acad. Sci.* **111**, 75–80 (2014).
